# Supplementary material for: Observation of 2e-periodic Supercurrents in Nanowire Single-Cooper-Pair Transistors
Source: arXiv:1805.10266 ancillary file (2018-05-25)
Supplement: Supplementary file 1 [file supplement_v1.pdf]

# Supplemental Material – Observation of 2$e$-periodic Supercurrents in Nanowire Single Cooper Pair Transistors

Jasper van Veen,[1,2] Alex Proutski,[1,2] Torsten Karzig,[3] Dmitry I. Pikulin,[3] Roman M. Lutchyn,[3] Jesper Nygård,[4] Peter Krogstrup,[5] Attila Geresdi,[1,2] Leo P. Kouwenhoven,[6,1,2] and John D. Watson[6,*]

[1]*QuTech, Delft University of Technology, 2600 GA Delft, The Netherlands*

[2]*Kavli Institute of Nanoscience, Delft University of Technology, 2600 GA Delft, The Netherlands*

[3]*Station Q, Microsoft Corporation, Santa Barbara, California 93106-6105, USA*

[4]*Center for Quantum Devices, Niels Bohr Institute, University of Copenhagen, 2100 Copenhagen, Denmark*

[5]*Center for Quantum Devices and Microsoft Quantum Lab Copenhagen, Niels Bohr Institute, University of Copenhagen, 2100 Copenhagen, Denmark*

[6]*Microsoft Station Q Delft, Delft University of Technology, 2600 GA Delft, The Netherlands*

(Dated: May 25, 2018)

TABLE S1: Device overview. Parameters characterizing the devices are the length of the island $L$, the thickness of the aluminum shell $t_{Al}$, and the backgate layout. Moreover, the geometric charging energy $E_C^0$ and superconducting gap $\Delta$ are listed. These parameters are extracted from charge stability diagrams in the strongly Coulomb blockaded regime (data shown in Figure S1). In addition, the cooldown at which the device was measured is specified.

| Device | $L$(µm) | Backgate layout | $t_{Al}$ (nm) | $E_C^0$ (meV) | $\Delta$(µeV) | Cooldown |
|---|---|---|---|---|---|---|
| 1 | 0.5 | Global | 5 | 1.5 | 0.18 | 2 |
| 2 | 1 | Global | 5 | 0.85 | 0.16 | 2 |
| 3 | 2 | Global | 5 | 0.44 | 0.22 | 2 |
| 4 | 3 | Global | 5 | 0.35 | 0.18 | 2 |
| 5 | 3 | Global | 5 | No data | No data | 2 |
| 6 | 1.2 | Local | 8 | 0.5 | 0.16 | 1 |

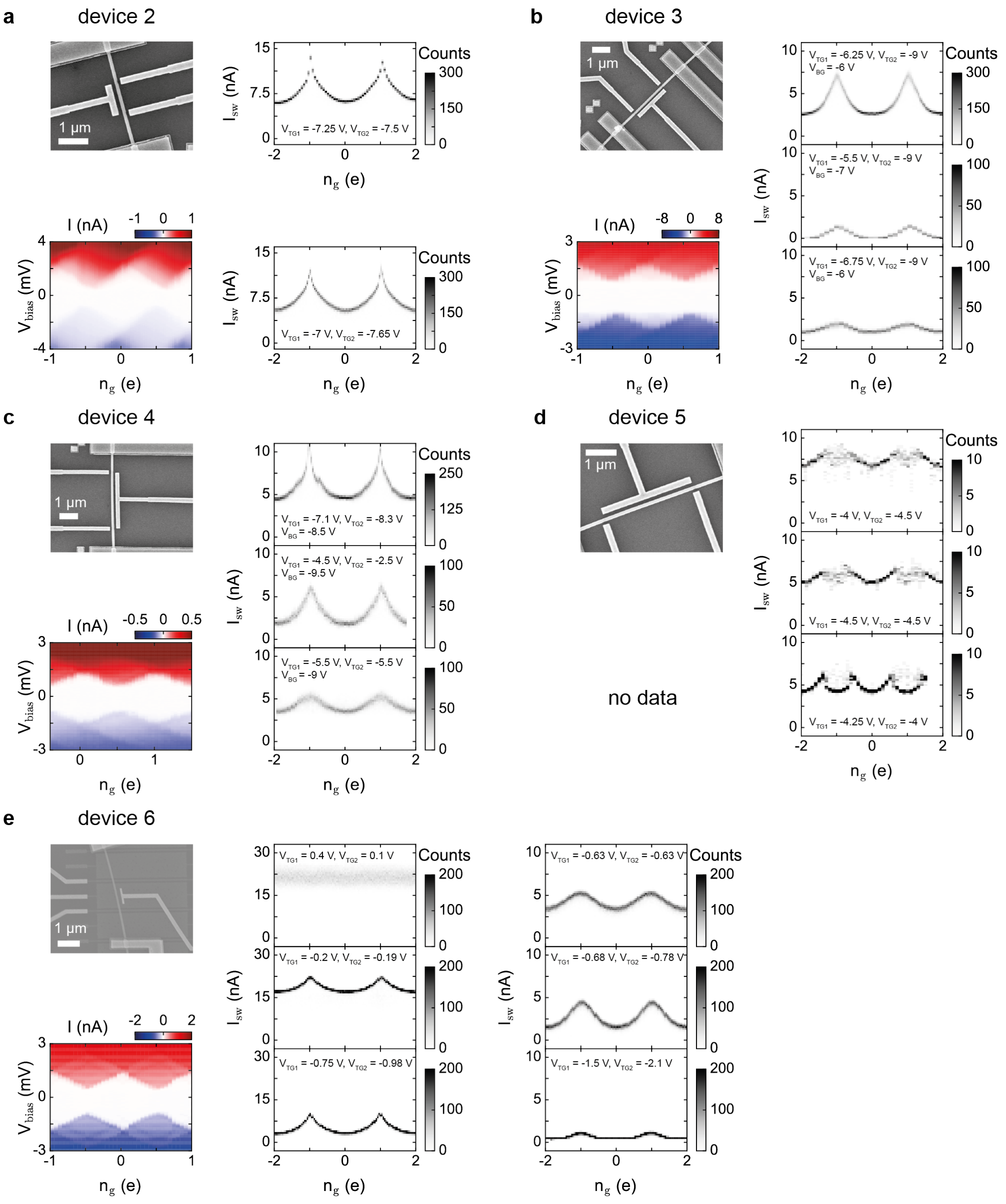


FIG. S1: Scanning electron micrographs, Coulomb blockade diamonds, and gate dependence of the $2e$-periodic signal for device 2-6 ($\mathbf{a}-\mathbf{e}$). The $E_C^0$ and $\Delta$ extracted from the Coulomb blockade data are summarized in Tabel S1. Note that apart from device 5 which shows an even-odd pattern in the switching current modulation, all devices show a $2e$ modulation, illustrating that the $2e$ signal does not correspond to a fine-tuned gate setting. The gate settings corresponding to the measurements are specified in each subfigure. The gates are labeled using the same convention as in the main text. For device 2, 5, and 6 the backgate is fixed at $V_{BG2}=-10$ V, $V_{BG5}=-8.5$ V, and $V_{BG6}=0$, respectively.

## I. OVERDAMPED JUNCTION LIMIT

In this section, we discuss the I-V characteristics and switching dynamics of overdamped junctions in the presence of quasiparticles. For larger temperatures where the I-V characteristics depart from $2e$ periodicity the junction is typically in the overdamped regime which allows the following theory to capture the $2e$ to $1e$ crossover (see Fig. 3 in the main text).

### A. Overdamped RCSJ model

We start with the standard RCSJ model of a junction with dissipative resistance $R_J$, capacitance $C$ and Josphenson energy $E_J = I_c\hbar/2e$. The overdamped regime is reached once the damping rate $\tau_R^{-1} = (R_J C)^{-1}$ exceeds the plasma frequency $\omega_p = \sqrt{2eI_c/\hbar C}$. The equation of motion then takes the form of the Langevin equation

$$\dot{\phi} + \sin\phi = \mathcal{I} + \sqrt{2\Gamma_T}\eta(t)\,, \tag{S1}$$

where $\phi$ is the phase differences across the junction, $\mathcal{I} = I_{\text{bias}}/I_c$ is the current bias relative to the critical current, and time is measured relative to $\tau_J = (2eI_cR_J/\hbar)^{-1} = \tau_R^{-1}\omega_p^{-2}$. Fluctuations due to thermal noise $\Gamma_T = k_BT/E_J$ are assumed to be short-time correlated $\langle\eta(0)\eta(t)\rangle = \delta(t)$. Note that in these units the renormalized voltage $v = V/I_cR_J$ is given by $v = \dot{\phi}$. The Langevin form can be mapped to a Fokker-Planck equation

$$\partial_t p = \partial_\phi\left([\partial_\phi u]p\right) + \Gamma_T\partial_\phi^2 p \tag{S2}$$

in terms of the probability distribution $p = p(\phi, t)$ and the potential $u(\phi, \mathcal{I}) = -\cos\phi - \mathcal{I}\phi$. Eq. (S2) is in the form of a continuity equation $\partial_t p + \partial_\phi j_p = 0$ which defines the probability current

$$j_p = -[\partial_\phi u]p - \Gamma_T\partial_\phi p\,. \tag{S3}$$

The I-V characteristics can be obtained from considering the stationary case $\partial_t p = 0$ of constant current $\partial_\phi j_p = 0$. When the probability distribution is normalized with respect to the interval $[0, 2\pi]$ using periodic boundary conditions in $\phi$, the current $j_p$ is a measure for the rate at which the phase particle traverses the interval and is therefore related to the

voltage $v = 2\pi j_p$. Solving Eq. (S3) yields the I-V characteristics [1–3]

$$v = 2\pi\Gamma_T \left(e^{\frac{2\pi\mathcal{I}}{\Gamma_T}} - 1\right) \left\{ \int_0^{2\pi} d\phi \left[ \int_0^{\phi} d\phi' + e^{\frac{2\pi\mathcal{I}}{\Gamma_T}} \int_{\phi}^{2\pi} d\phi' \right] e^{\frac{u(\phi',\mathcal{I}) - u(\phi,\mathcal{I})}{\Gamma_T}} \right\}^{-1} . \quad \text{(S4)}$$

### B. Quasiparticle dynamics in the overdamped RCSJ model

The overdamped RCSJ model can be readily extended to include quasiparticle dynamics by keeping track of the even $\alpha = 0$ and odd $\alpha = 1$ state of the island,

$$\partial_t \begin{pmatrix} p_0 \\ p_1 \end{pmatrix} + \partial_\phi \begin{pmatrix} j_0 \\ j_1 \end{pmatrix} = \begin{pmatrix} -\gamma_{\text{in}} p_0 + \gamma_{\text{out}} p_1 \\ +\gamma_{\text{in}} p_0 - \gamma_{\text{out}} p_1 \end{pmatrix} , \quad \text{(S5)}$$

where $j_\alpha = -[\partial_\phi u_\alpha]p - \Gamma_T \partial_\phi p_\alpha$ in terms of the parity dependent potential $u_\alpha(\phi, \mathcal{I}) = -a_\alpha \cos\phi - \mathcal{I}\phi$ with $a_0 = 1$ and $a_1 = E_{J1}/E_{J0}$. Here $\gamma_{\text{in/out}} = \Gamma_{\text{in/out}}\tau_J$ are dimensionless rates of switching the system from even to odd or vice versa. To derive the I-V characteristics we again look at the steady state $\partial_t p_0 = \partial_t p_1 = 0$. We then observe that $\partial_\phi(j_0 + j_1) = 0$ and, similar to the single state case, the constant is fixed by the voltage $j_0 + j_1 = v/2\pi$. The normalization condition of the probabilities is now in terms of $\int d\phi(p_0 + p_1) = \bar{p}_0 + \bar{p}_1 = 1$. We now consider the two limiting cases of slow and fast poisoning.

#### *1. Slow poisoning limit*

In the slow poisoning limit corresponding to $\gamma_{\text{in}}, \gamma_{\text{out}} \ll 1$ the right hand side of Eq. (S5) can be neglected which, in the steady state, sets both $j_0$ and $j_1$ independently to a constant and therefore recovers the standard RCSJ model. The result from Sec. (I A) can essentially be copied with voltages $v_\alpha$ defined by Eq. (S4) using the potential $u_\alpha$ of the corresponding parity state. To calculate the total voltage drop one needs to take into account that the normalization of the probabilities $\int_0^{2\pi} d\phi p_{0/1} = \bar{p}_{0/1} = \gamma_{\text{out/in}}/(\gamma_{\text{out}} + \gamma_{\text{in}})$ enters Eq. (S4) so that the voltages $v_\alpha$ are correctly weighted. This yields

$$v = v_0 \bar{p}_0 + v_1 \bar{p}_1 . \quad \text{(S6)}$$

We therefore conclude that in the slow poisoning case the I-V characteristic is the weighted sum of the I-V characteristics of each parity where the weight is given by the average occupation. For significantly different even and odd switching currents we would therefore expect

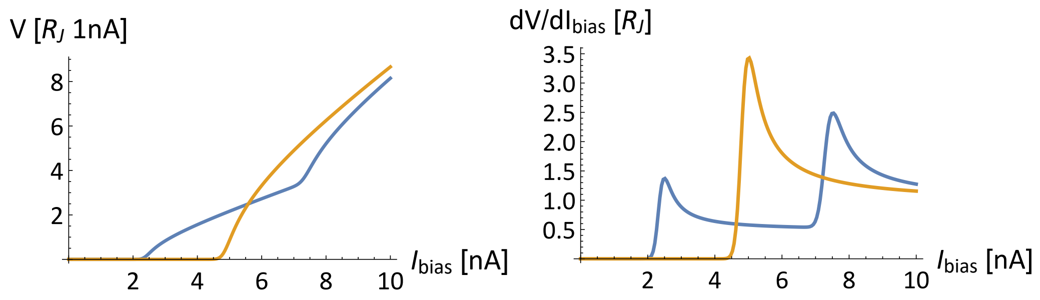


FIG. S2: Analytic solution of the slow and fast poisoning limit. Voltage drop $V$ in terms of the bias current $I_{\text{bias}}$ (left) and $dV/dI_{\text{bias}}$ (right). The slow poisoning case (blue) is showing a double-kink behavior while fast poisoning (yellow) leads to a single-kink at the averaged switching current. Parameters are $I_c^{(0)} = 2.5\text{nA}$, $I_c^{(1)} = 7.5\text{nA}$, and $\Gamma_T = 0.05$.

a double-kink in the I-V characteristics which is most clearly visible in the derivative $dV/dI$ which subsequently turns into a double-peak (see Fig. S2).

### 2. *Fast poisoning limit*

In the fast poisoning limit corresponding to $\gamma_{\text{in}}, \gamma_{\text{out}} \gg 1$ the probabilities $p_\alpha(\phi)$ have to cancel the leading order of the right hand side of Eq. (S5) [up to terms $\mathcal{O}(1)$]. This allows to separate the fast quasiparticle dynamics, that lock the ratio of $p_0(\phi)/p_1(\phi)$ to $\bar{p}_0/\bar{p}_1$ for each $\phi$, from the $\phi$-dependence of the probability distribution, i.e. use the ansatz $p_\alpha(\phi) = \bar{p}_\alpha p_+(\phi)$ with $p_+(\phi) = p_0(\phi) + p_1(\phi)$. We can then solve for $p_+(\phi)$ by looking at the sum of both components of Eq. (S5)

$$\begin{aligned}\frac{v}{2\pi} = j_1 + j_2 &= -[\partial_\phi u_0]p_0 - [\partial_\phi u_1]p_1 - \Gamma_T \partial_\phi (p_0 + p_1) \\ &= -[\partial_\phi (\bar{p}_0 u_0 + \bar{p}_1 u_1)]p_+ - \Gamma_T \partial_\phi p_+ \,,\end{aligned}$$

which yields the same type of equation to solve as for the standard RCSJ model with an effective potential $u_{\text{eff}} = \bar{p}_0 u_0 + \bar{p}_1 u_1$. The solution corresponds to a single kink that signals the onset of the resistive state that lies in between the double step kink solution of the slow poisoning case, see Fig. S2.

### *3. General case*

In the general case the differential equation (S5) can be solved numerically. Figure S3 shows a gray scale plot of the dV/dI-I characteristics for fast/intermediate/slow poisoning with different in/out rate ratios. Comparing the different poisoning scenarios with the experimental data of Fig. 3 clearly shows that at high temperatures, where the $\Gamma_{\rm in}/\Gamma_{\rm out}$ ratio is sizable, slow and intermediate poisoning is incompatible with the experimental data while fast poisoning yields an excellent agreement. Note that at the level of Eq. (S5) the critical currents $I_{\rm c}^{(\alpha)}(n_g)$ are input parameters. For simplicity, we used a parabolic dependence with a minimum and maximum of 2.5nA and 7.5nA to resemble the behavior of Fig. 2b in the main text.

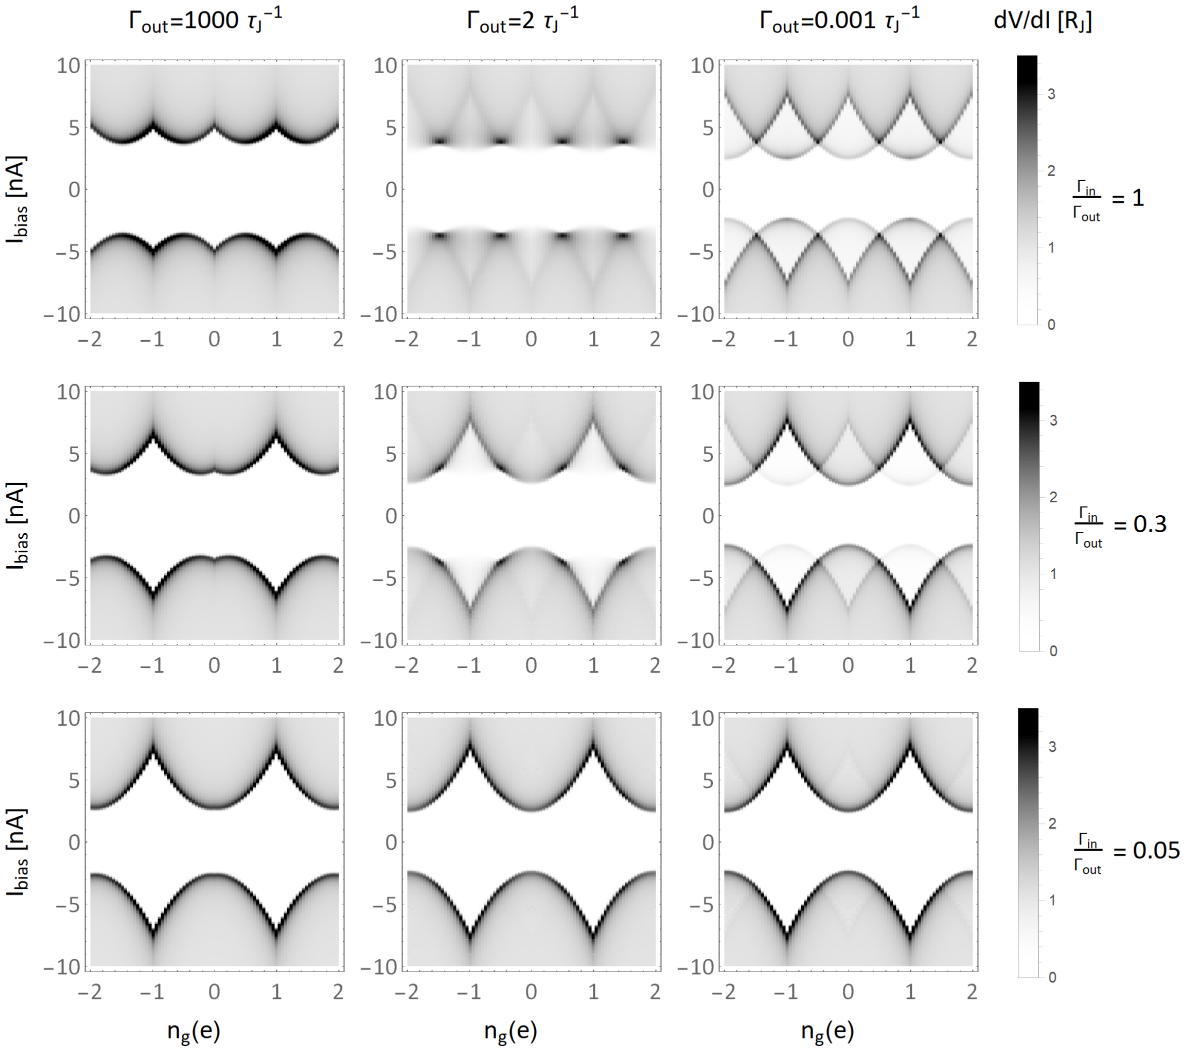


FIG. S3: Numerical solution of the dV/dI characteristics in different parameter regimes. The columns from left to right correspond to fast, intermediate and slow poisoning, respectively. The rows correspond to different ratios of $\Gamma_{in}/\Gamma_{out}$ and are therefore a measure of the temperature. For concreteness the plots assume a fixed ratio corresponding to a weak charge dispersion.

## II. TEMPERATURE DEPENDENCE

In this section, we discuss the model used to fit the switching current histograms in Fig. 3 of the main text for varying temperature. In our model, we assume that the quasiparticle poisoning and unpoisoning rate is fast compared to the characteristic switching time of the junction $\Gamma_{\text{in}}, \Gamma_{\text{out}} \gg 1/\tau_J$. Under this assumption, which is justified above in Section I, the critical current of the SCPT is given by the weighted average of the critical currents in the even and odd states with the weighting coefficients given by the free energy difference between the parity states of the SCPT. In the opposite regime when the switching rate of the junction is much larger than the poisoning or unpoisoning rate $\Gamma_{\text{in}} \ll 1/\tau_J$ or $\Gamma_{\text{out}} \ll 1/\tau_J$, we expect a bimodal switching current distribution. This is not observed in the temperature dependence data. It is important to note that the fast poisoning-unpoisoning assumption may be broken at small temperatures, where the probability of odd state occupation is very small. Even though we do not see bimodal distribution of the switching current at low temperatures, this may be due to weak spectral density of the peak corresponding to the odd occupations.

Thus, we need to compute the critical currents in the two parity states as functions of the gate charge $n_g$, as well as the free energy difference between the two states. We start with the Hamiltonian of the system which consists of three terms: $H_J + H_C + H_{\text{BCS}}$. The Josephson term has the form

$$H_J = E_{J1}\cos(\hat{\varphi}_i - \phi/2) + E_{J2}\cos(\hat{\varphi}_i + \phi/2), \tag{S7}$$

where $E_{J1,2}$ are the Josephson energies of the two junctions, $\hat{\varphi}_i$ is the superconducting phase of the island, and $\phi$ is the phase difference between the superconducting leads. This expression can be rewritten as

$$H_J = (E_{J1} + E_{J2})\sqrt{1 - \frac{4E_{J1}E_{J2}}{(E_{J1} + E_{J2})^2}\sin^2\phi/2}\,\cos(\hat{\varphi}_i - \varphi_0), \tag{S8}$$

where $\varphi_0$ is a $E_{J1,2}$-dependent constant. We notice that the operator $e^{i\hat{\varphi}_i}$ changes the number of particles on the island by two, thus the Josephson Hamiltonian in the charge basis $|n\rangle$ can be written as

$$H_J = (E_{J1} + E_{J2})\sqrt{1 - \frac{4E_{J1}E_{J2}}{(E_{J1} + E_{J2})^2}\sin^2\phi/2}\sum_n |n\rangle\langle n+2| + \text{h. c.} \tag{S9}$$

For the fitting procedure we fix moderately asymmetric junction with $E_{J1}/E_{J2} = 2$. Moreover, the Josephson energy in the main text is defined as $H_J(\phi = 0) - H_J(\phi = \pi)$.

Next, the Coulomb term of the Hamiltonian is given by

$$H_C = \sum_n E_C(n - n_g)^2 |n\rangle\langle n|, \tag{S10}$$

where $E_C = e^2/2C$ with $e$ the elementary electron charge and $C$ the effective capacitance of the island taking into account the geometric capacitance and possible renormalization effects due to (virtual) tunneling of quasiparticles. Finally, we approximate the energy to add an unpaired quasiparticle to the superconducting island as

$$H_{\mathrm{BCS}} \approx \sum_n \Delta \frac{1 - (-1)^n}{2} |n\rangle\langle n|, \tag{S11}$$

where $\Delta$ is the superconducting gap on the island, and $\frac{1-(-1)^n}{2}$ is the parity of the SCPT. The approximation corresponds to the limit of small typical excitation energies of quasiparticles relative to the gap edge $\Delta$. Note that while this approach captures the dominant contribution to the energetics, it is important to include the full quasiparticle dispersion for the entropic contribution discussed below.

Using the total Hamiltonian $H = H_J + H_C + H_{\mathrm{BCS}}$ in the even parity sector, we can find the even ground state energy of the SCPT as a function of the phase difference between the superconducting leads $\phi$ and gate charge $n_g$, $E^{\mathrm{even}}(\phi, n_g)$. The odd ground state energy is found by shifting $E^{\mathrm{even}}(\phi, n_g)$ by $n_g = 1$ and adding the superconducting gap; $E^{\mathrm{odd}}(\phi, n_g)$ $= E^{\mathrm{even}}(\phi, n_g + 1) + \Delta$. The zero-temperature supercurrent is given by the derivative of the ground state energy as a function of phase difference

$$I_c^{\mathrm{even}}(\phi, n_g) = \frac{e}{\hbar} \frac{\partial}{\partial \phi} E^{\mathrm{even}}(\phi, n_g)\,. \tag{S12}$$

The finite-temperature supercurrent is given by the weighted sum of the even and odd ones with the assumption of the fast (un)poisoning, where the weighting factors $p_{\mathrm{odd}}$ and $p_{\mathrm{even}} = 1 - p_{\mathrm{even}}$ are calculated as follows

$$p_{\mathrm{odd}}(T, \phi, n_g) = \frac{Z_{\mathrm{odd}}}{Z_{\mathrm{even}} + Z_{\mathrm{odd}}} = \frac{1}{1 + \exp(\Delta F(T, \phi, n_g)/k_B T)}, \tag{S13}$$

where $Z_{\mathrm{odd,even}}$ are the partition functions in the state with and without a quasiparticle on the middle island, respectively, $\Delta F$ is the free energy difference between the parity states, $k_B$ is the Boltzmann constant, and $T$ is the temperature.

The free energy difference between the two parity states can be computed as follows

$$\Delta F(T, \phi, n_g) = \delta E(\phi, n_g) - T \ln \tanh z_i(T, \delta_i), \tag{S14}$$

$$z_i(T, \delta_i) = \frac{2\pi\sqrt{k_B T \Delta}}{\delta_i} \exp(-\Delta/k_B T). \tag{S15}$$

Here $\delta E(\phi, n_g) = E^{\text{even}}(\phi, n_g + 1) - E^{\text{even}}(\phi, n_g)$ is the difference in ground state energy between the odd and even parity sectors (not including $\Delta$),

$z_i$ is the partition function difference between the quasiparticle being inside the island at energy $\Delta$ and in the lead at zero energy, and $\delta_i$ is the level spacing inside the island. In this expression we assume that the quasiparticle is tunneling from a gapless, large quasiparticle trap. This means the lead has negligible level spacing and negligible change of entropy due to the removal of one electron from the trap. We assume $\delta_i = 5$mK. This gives the following expression which we use to fit the data

$$I_c(T, n_g) = \max_{\phi} \left[ I_c^{\text{even}}(\phi, n_g)(1 - p_{\text{odd}}(T, \phi, n_g)) + I_c^{\text{even}}(\phi, n_g + 1) p_{\text{odd}}(T, \phi, n_g) \right]. \tag{S16}$$

Equation (S16) fits the data nicely, as shown in Fig. 3a of the main text. It is important to mention that the same fit assuming non-equilibrium quasiparticles in the lead instead of equilibrium quasiparticles in the trap does not fit the data, since even at lowest temperatures it would produce even-odd or purely 1e periodicity. We thus conclude that the dominating poisoning effect is via direct tunneling of the quasiparticles from the normal lead.

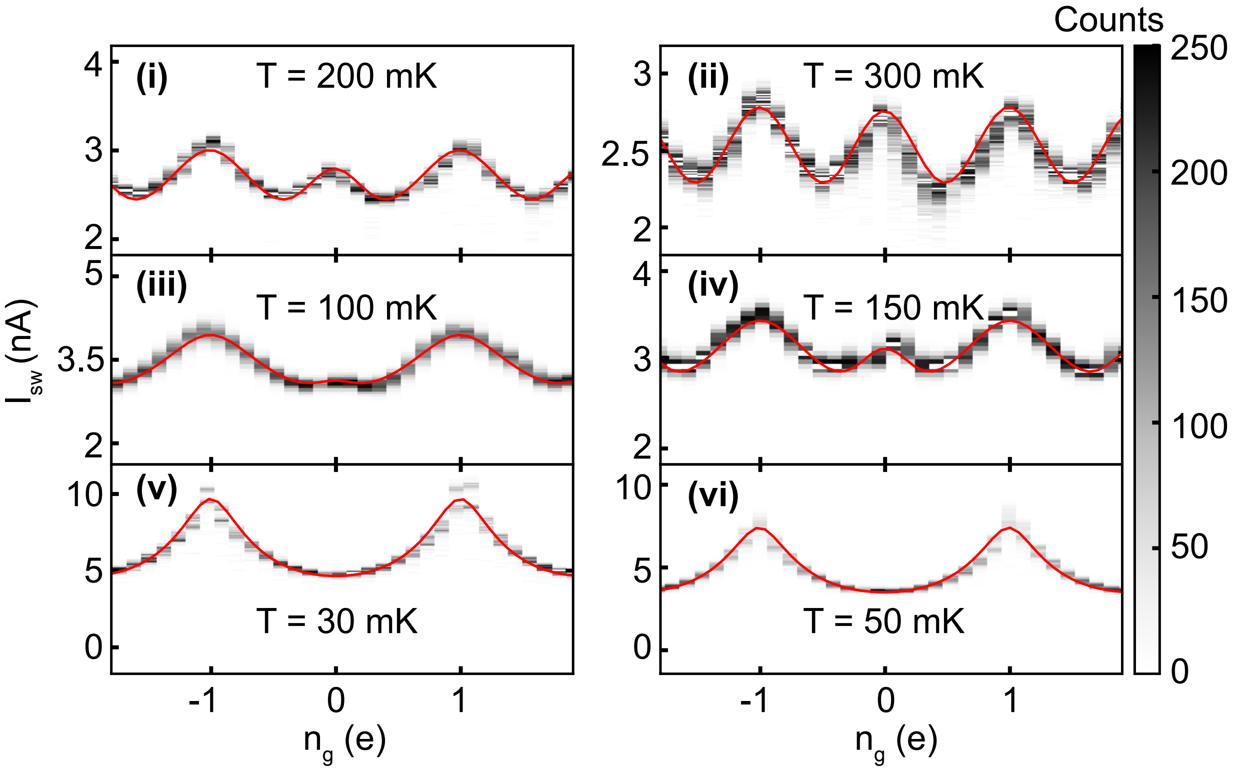


FIG. S4: Switching current modulation as a function of temperature for device 2 at $R_N = 10.5\,\mathrm{k\Omega}$. The experimental histograms shown in grayscale are overlaid by the theoretical fit to the average switching current $\langle I_{\mathrm{sw}} \rangle$ (red curves). Individual fits are for different values of $\Delta$, $E_J$, and $E_C$. The resulting values for the parameters are $\Delta \approx 245\,\mathrm{\mu eV}$, $E_C \approx 192\,\mathrm{\mu eV}$, and $E_J \approx 111\,\mathrm{\mu eV}$.

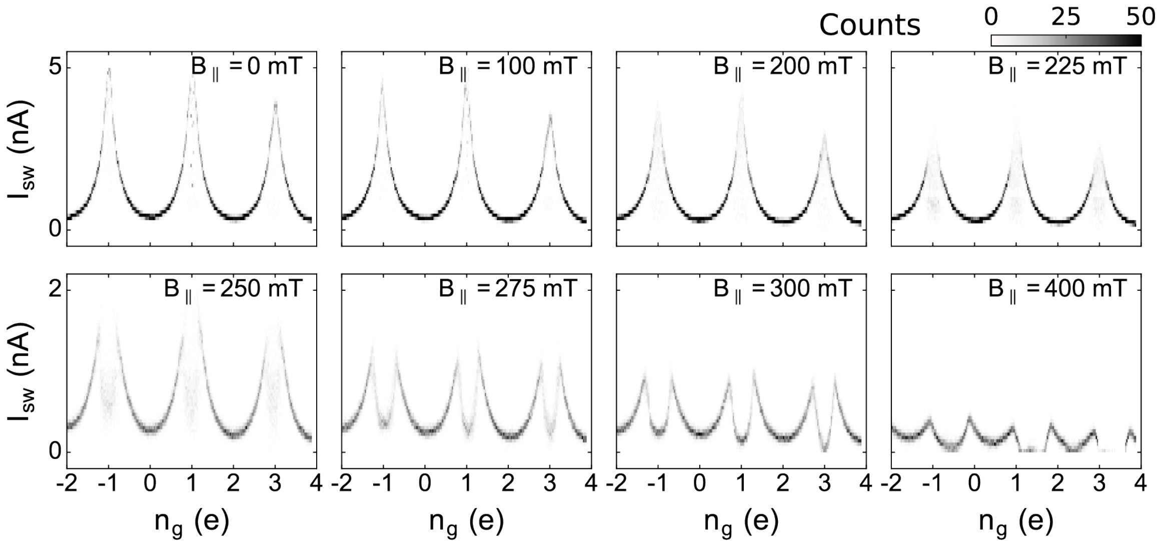


FIG. S5: Representative switching current histograms as a function of parallel magnetic field for device 1 at $V_{BG} = -7.55$ V, $V_{TG1} = V_{TG2} = -1.5$ V. The $S_{\rm even}$ and $S_{\rm odd}$ spacings reported in Figure 4e are extracted from the average $S_{\rm even}$ and $S_{\rm odd}$ of these histograms. Note that the histogram at $B_{\parallel} = 400$ mT is distorted around $n_g = 1.5$ and $n_g = 3.5$ due to false triggers.

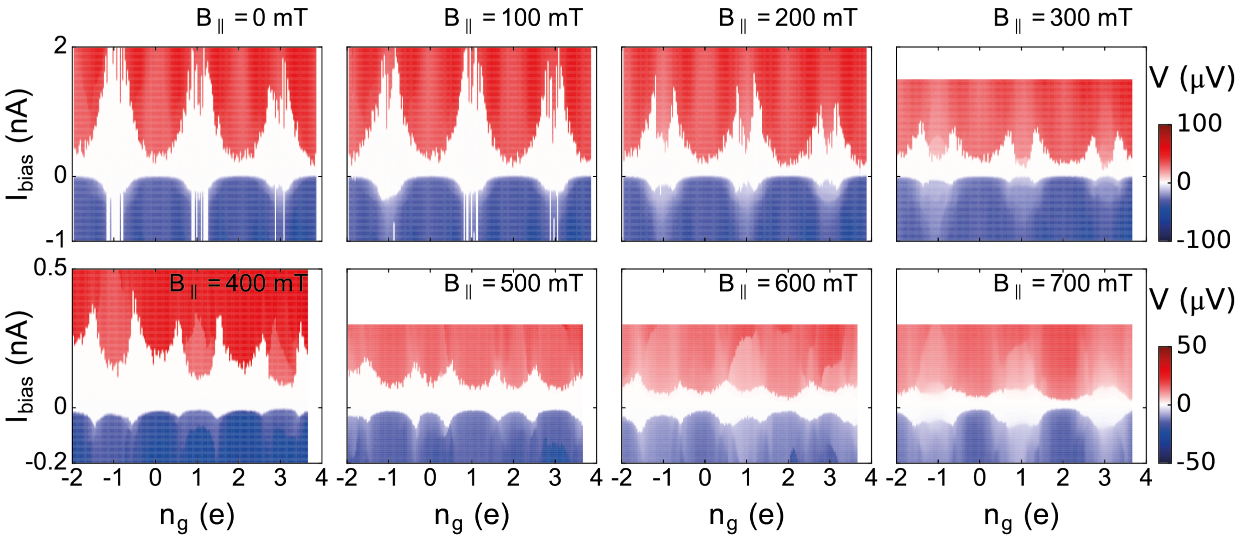


FIG. S6: Representative I-V characteristics as a function of parallel magnetic field for device 1 at $V_{BG} = -7.55$ V, $V_{TG1} = V_{TG2} = -1.5$ V. The $S_{\rm even}$ and $S_{\rm odd}$ spacings reported in Figure 4e are extracted from the average $S_{\rm even}$ and $S_{\rm odd}$ of these I-V characteristics.

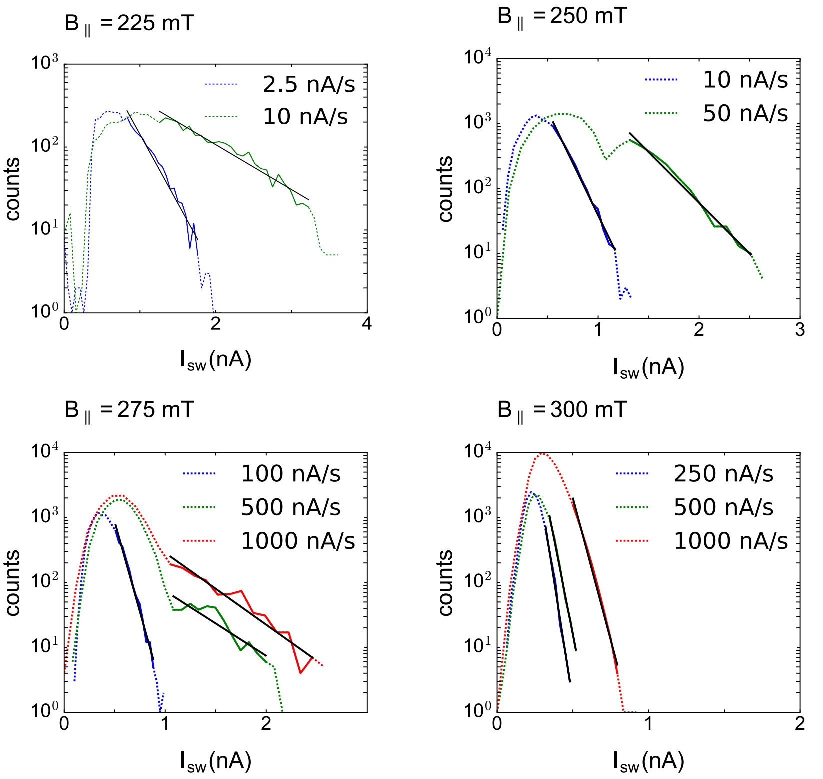


FIG. S7: Slow switching current histograms at $n_g = 1$ at representative values of the magnetic field taken on device 1 at $V_{BG} = -7.55$ V, $V_{TG1} = V_{TG2} = -1.5$. The even state lifetime $\tau_{\rm even}$, presented in Figure 4f of the main text, was obtained from the exponential tail of the histograms, using the following model: $N = N_0 \exp\left(-\frac{I-I_0}{dI/dt\tau_{\rm even}}\right)$, where $N_0$ is the number of counts at $I_0$ and $dI/dt$ is the current ramp rate. The extracted lifetimes are tabulated in Table S2.

TABLE S2: Overview of the even state lifetimes at $n_g = 1$ as a function of the parallel magnetic field $B_{\parallel}$ taken on device 1, this data is presented in Figure 4f of the main text. In addition, the current ramp rate $dI/dt$ and the sample size $N$ used to construct the switching current histogram are presented.

| $B_{\parallel}$ (mT) | $dI/dt$ (nA/s) | $\tau_{\text{even}}$ (ms) | $N$ |
|---|---|---|---|
| 225 | | | |
| | 2.5 | 105 | 3500 |
| | 10 | 80 | 5000 |
| 237 | | | |
| | 2.5 | 50 | 5000 |
| | 10 | 30 | 10000 |
| 250 | | | |
| | 10 | 4.8 | 10000 |
| | 50 | 5.6 | 10000 |
| 262 | | | |
| | 50 | 1.6 | 10000 |
| | 100 | 2.4 | 25000 |
| 275 | | | |
| | 100 | 0.78 | 10000 |
| | 500 | 0.87 | 10000 |
| | 1000 | 0.39 | 10000 |
| 287 | | | |
| | 500 | 0.1 | 10000 |
| | 1000 | 0.26 | 50000 |
| | 2000 | 0.22 | 50000 |
| 300 | | | |
| | 250 | 0.11 | 10000 |
| | 500 | 0.073 | 10000 |
| | 1000 | 0.05 | 50000 |

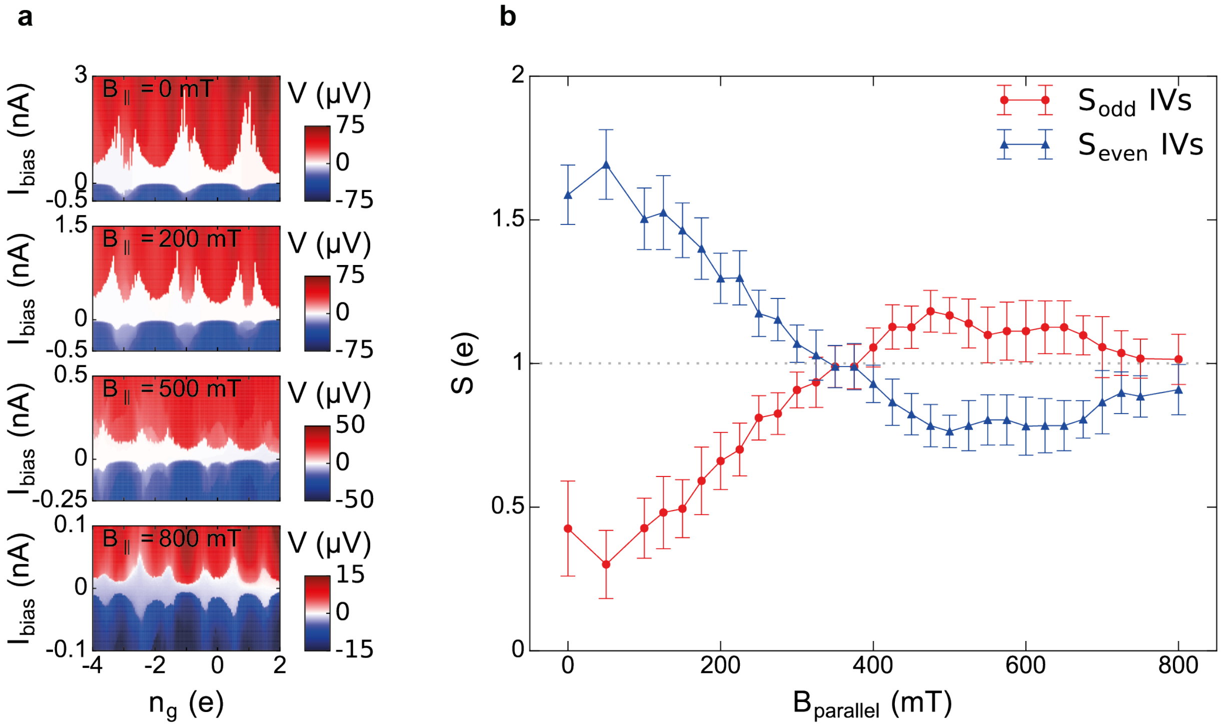


FIG. S8: Parallel magnetic field dependence of the even and odd spacing in device 1 at $V_{BG} = -7.65$ V, $V_{TG1} = V_{TG2} = -1.5$ V. Although it is very close to the used gate setting for the data presented in Figure 4 of the main text, we believe this corresponds to a different charge configuration in the SCPT because the of hysteresis in the gate response. **(a)** I-V characteristic used for the construction of **(b)** for representative values of the parallel magnetic field. **(b)** $S_{even}$ and $S_{odd}$ as a function of the parallel magnetic field. $S_{even}$ ($S_{odd}$) is obtained by averaging over 2 (3) succesive spacings respectively. At this gate setting, the spacings also cross confirming the data presented in Figure 4e of the main text. However, the shape of the oscillation pattern is different from Figure 4e.

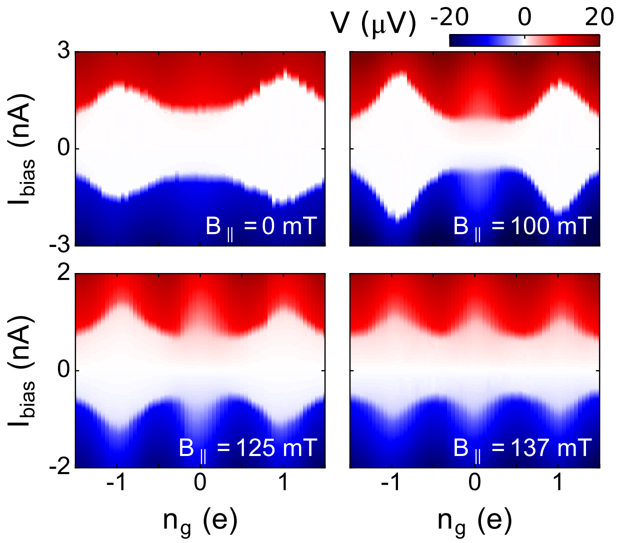


FIG. S9: Parallel magnetic field dependence of the I-V characteristics of device 4. Instead of an even-odd pattern that develops as a function of field as was observed for device 1, the I-V characteristics develops a peak in the switching current at odd gate charge similar to the behavior that was observed as a function of temperature. This indicates that the SCPT is in the fast unpoisoning limit possibly caused by a field-induced softening of the gap.

---


* To whom correspondence should be addressed; E-mail: john.watson@microsoft.com



[1] Y. M. Ivanchenko and L. A. Zil'Berman, JETP **28**, 113 (1969).

[2] V. Ambegaokar and B. I. Halperin, Phys. Rev. Lett. **22**, 1364 (1969).

[3] Likharev, *Dynamics of Josephson Junctions and Circuits* (CRC Press, 1986).
